# Supplementary material for: DIAR: Removing Uninteresting Bytes from Seeds in Software Fuzzing
Source: arXiv:2112.13297 source file (2021-12-25)
Supplement: Supplementary file 1 [file appendix.tex]

\section*{A. Using FMViz}
%Since we already used the term "Demonstration" in the main text

In this section, we describe the steps to run the first release of FMViz, version 1.0. We use libxml2 as our fuzzing test subject. All commands provided next are for the Linux environment.

\subsection*{Setting up the Environment}

\noindent\textit{1. FMViz Setup}

\vspace{5.5pt}

\noindent In any directory, we clone the FMViz repository as follows\footnote{Currently, the name of the repository has been purposely kept different from FMViz.}:

\vspace{5.5pt}

\noindent\hllg{\texttt{git clone --recursive git@github.com:AftabHussain/afl-test-viz.git}}

\vspace{5.5pt}

\noindent Then we build and install the AFL fuzzer, patched with FMViz's Test Input Color Representation Generator component, by performing the following command:

\vspace{5.5pt}

\noindent\hllg{\texttt{cd afl-test-viz/code/AFL-mut-viz/AFL \&\& make -j32 \&\& make install}}

\vspace{8.5pt}

\noindent\textit{2. \texttt{libxml2} Setup}

\vspace{5.5pt}

\noindent Once we have setup the fuzzer, we build the test subject (\texttt{libxml2}) with AFL's compiler (\texttt{afl-gcc}), which prepares \texttt{libxml2} binaries as fuzzing targets. We first obtain \texttt{libxml2} as follows in a folder outside \texttt{afl-test-viz} directory: 

\vspace{5.5pt}

\noindent\hllg{\texttt{git clone https://github.com/GNOME/libxml2.git \&\& cd libxml2 \&\& git checkout 1fbcf40}}

\vspace{5.5pt}

\noindent Finally, we configure and build \texttt{libxml2} by performing the following command:

\vspace{5.5pt}

\noindent\hllg{\texttt{cd libxml2 \&\& export CC=afl-gcc \&\& ./autogen.sh \&\& make -j32}}

\subsection*{Generating Color Representations of Test Inputs}

We now invoke the first part of FMViz, the augmented AFL fuzzer, which produces color representations (in hex) of test inputs generated while fuzzing the test subject. In this demo, we fuzz the \texttt{libxml2} binary, \texttt{xmllint}. We thus enter the \texttt{libxml2} folder, create an input folder (\texttt{input}), and place in it any XML file as a test input (some sample inputs are available in the FMViz repository):

\vspace{5.5pt}

\noindent\hllg{\texttt{cd libxml2 \&\& mkdir input \&\& cp [path\_to\_xml\_file] input/}}

\vspace{5.5pt}

\noindent Thereafter, we invoke the fuzzer as follows:   

\vspace{5.5pt}

\noindent\hllg{\texttt{export AFL\_SKIP\_CPUFREQ=1 \&\& export LD\_LIBRARY\_PATH=./.libs/ \&\& \\afl-fuzz -i input/ -o output/  -- ./.libs/xmllint -o /dev/null @@}}

\vspace{5.5pt}

\noindent The fuzzing process can be terminated anytime using \texttt{Ctrl+C} -- on termination all results are saved in the output folder, \texttt{output}. Inside this folder, the color dump file \texttt{tests\_generated} contains color representations of all the tests created by the fuzzer. 

\subsection*{Generating Images from Color Representations of Test Inputs}

To generate test input images, we process the color dump file obtained in the previous phase. We place this file along with the Image Generation program (\texttt{viz\_tests.py}) in a separate directory:

\vspace{5.5pt}

\noindent\hllg{\texttt{mkdir process\_color\_rep}}

\vspace{5.5pt}

\noindent\hllg{\texttt{cp libxml2/output/tests\_generated process\_color\_rep/}}

\vspace{5.5pt}

\noindent\hllg{\texttt{cp afl-test-viz/code/viz\_tests.py process\_color\_rep/}}

\vspace{5.5pt}

\noindent Finally we invoke the script:

\vspace{5.5pt}

\noindent\hllg{\texttt{cd process\_color\_rep/ \&\& python viz\_tests.py}}

\vspace{5.5pt}

\noindent The above command generates PNG images for all tests, that are represented in the color dump file, in \texttt{process\_color\_rep} directory:

\vspace{5.5pt}

\noindent\hllg{\texttt{ls | xargs -n 1}}

\vspace{-9.5pt}

\begin{verbatim}
.
.
.
file_000005564.png
file_000005565.png
file_000005566.png
file_000005567.png
file_000005568.png
file_000005569.png
file_000005570.png
file_000005571.png
file_000005572.png
.
.
\end{verbatim}

\begin{figure}[htbp]
  \centering
  
  \includesvg{figs/image-viewer-screen-shot}
  \caption{Screenshot of a test input image on Image Viewer}
  \label{fig-imgv-sshot}
\end{figure}

 \noindent A sample screenshot of a test input image, opened with Image Viewer, a default image viewer in Ubuntu, is shown in Figure~\ref{fig-imgv-sshot}. Since the image files for the input tests are named in the order in which they were produced during fuzzing, toggling over consecutive images in the image viewer application shows the trends in mutations. In order to produce a time-lapse video, we use Simple Screen Recorder~\cite{simplescreenrec}, which once installed can be invoked by the command \texttt{simplescreenrecorder} on the terminal. Then by starting recording and toggling over multiple images on Image Viewer by holding the left/right arrow key, we are able to record the mutation transitions that take place.
